# Supplementary material for: Incorporating Heterophily into Graph Neural Networks for Graph Classification
Source: arXiv:2203.07678 source file (2024-05-09)
Supplement: Supplementary file 1 [file sec_appendix.tex]

\section*{APPENDIX}

\subsubsection{homophily ratio $\alpha_v$}\label{sec:appendix1}

% \begin{figure*}[!htb]
% 	\centering
% 	\subfigure{\includegraphics [width=0.7\textwidth]{image/data1.pdf}}
	
% 	\centering
% 	\subfigure{\includegraphics [width=0.7\textwidth]{image/data2.pdf}}
	
% 	\centering
% 	\subfigure{\includegraphics [width=0.7\textwidth]{image/data3.pdf}}
% 	\caption{Illustration of the histogram of the homophily ratio $\alpha_v$ of nodes in each dataset. The x-axis denotes the value of $\alpha_v$ and the y-axis denotes the frequency (not shown here for clarity).}
% 	\label{fig:distributions}
% \end{figure*}
